# Supplementary material for: MiNL: Micro-images based Neural Representation for Light Fields
Source: arXiv:2209.08277 source file (2022-09-17)
Supplement: Supplementary file 1 [file appendix.pdf]

## 487 A Appendix

### 488 A.1 Results on different light field images

489 We perform experiments on different light field images (*i.e.* Danger\_de\_Mort, Stone\_Pillars\_Outside  
490 and Fountain&Vincent2) to validate the superiority of MiNL, as demonstrated by the following results  
491 on light field compression.

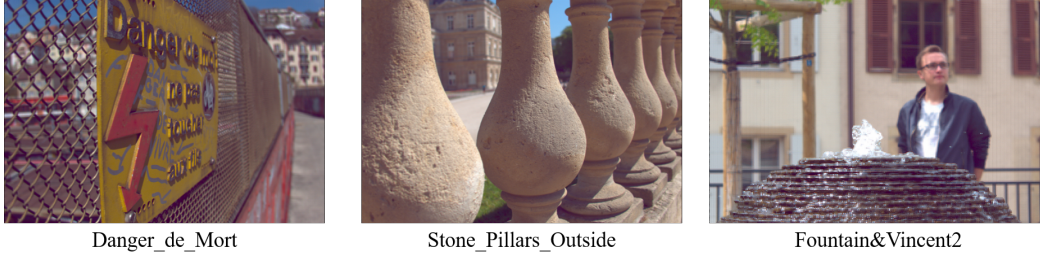

Figure 8: Different light field images used in our experiments

### 492 Danger\_de\_Mort

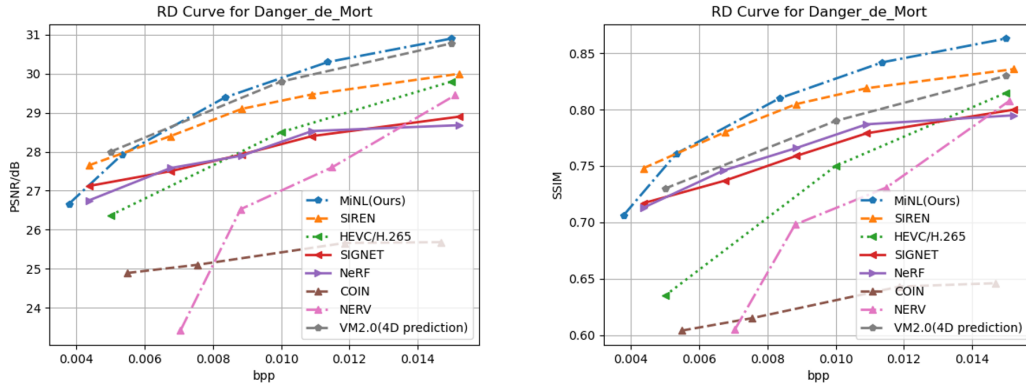

Figure 9: Light field compression results of different methods on Danger\_de\_Mort

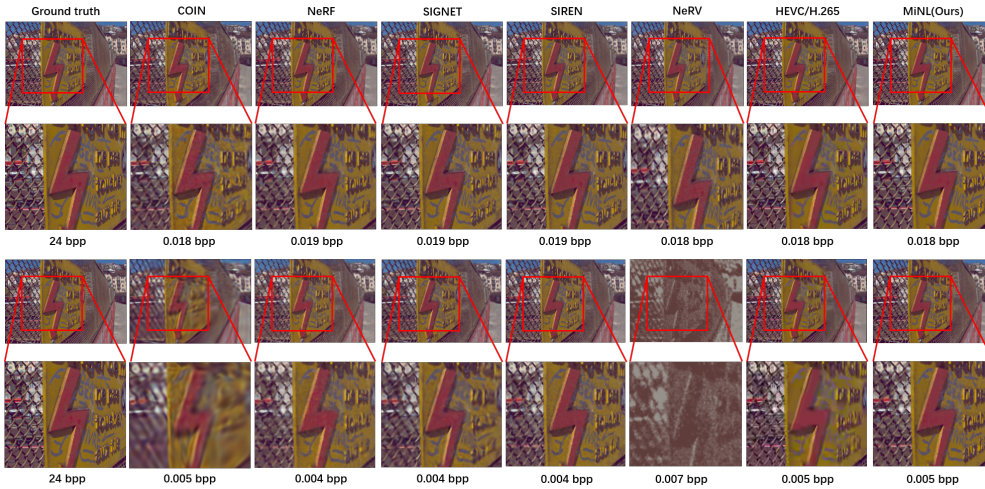

Figure 10: Visualization of light field compression results of different methods on Danger\_de\_Mort

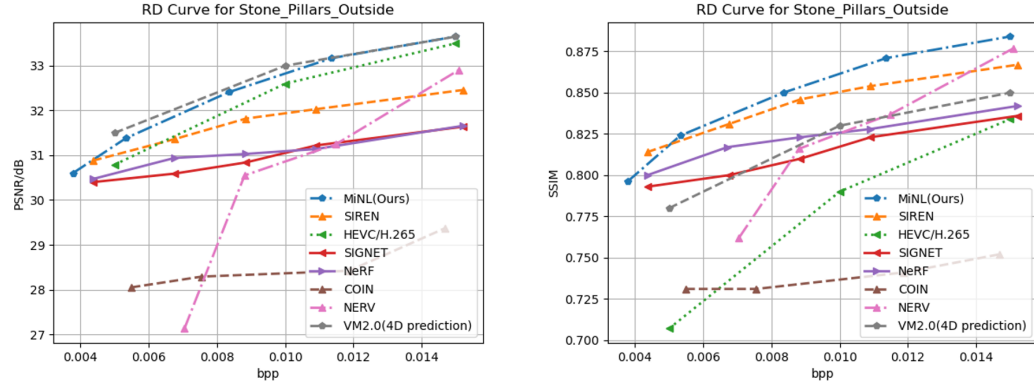

Figure 11: Light field compression results of different methods on Stone\_Pillars\_Outside

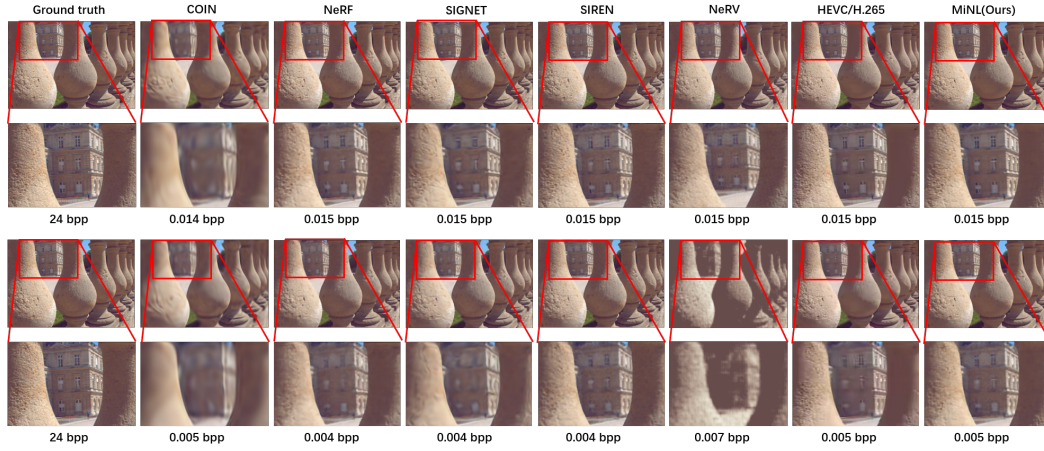

Figure 12: Visualization of light field compression results of different methods on Stone\_Pillars\_Outside

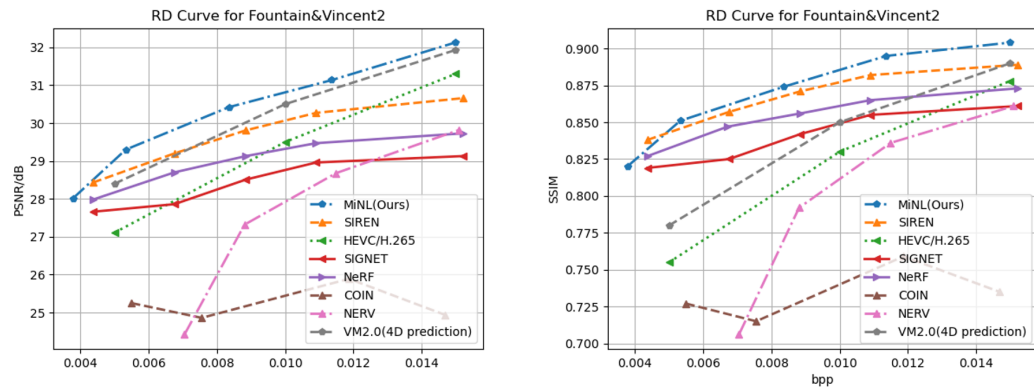

Figure 13: Light field compression results of different methods on Fountain&amp;Vincent2

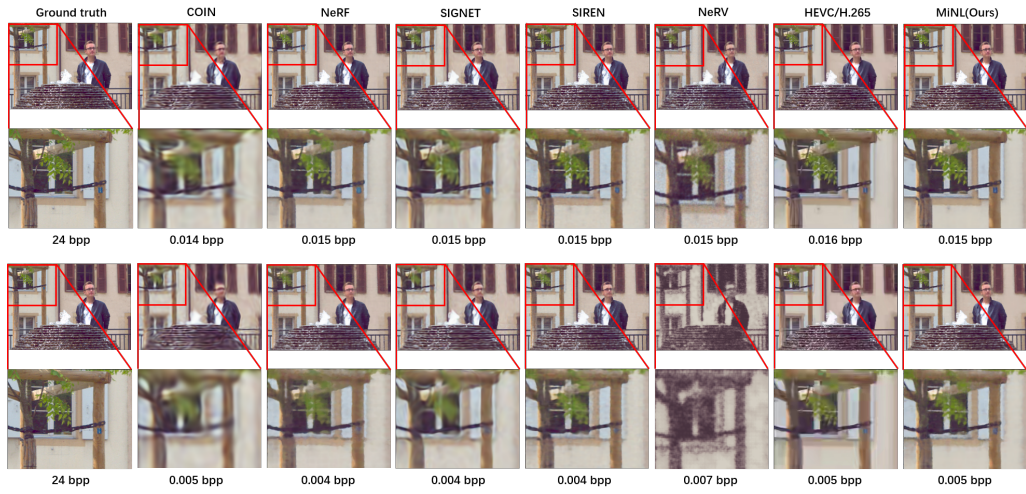

Figure 14: Visualization of light field compression results of different methods on Fountain&Vincent2
